# Supplementary material for: Predicting properties of hard-coating alloys using ab-initio and machine learning methods
Source: arXiv:2111.01111 source file (2021-11-23)
Supplement: Supplementary file 1 [file supplement.pdf]

# Supplementary: Predicting properties of hard-coating alloys using *ab-initio* and machine learning methods

H. Levämäki,[1,*] F. Tasnadi,[1] D. G. Sangiovanni,[1] L. J. S. Johnson,[2] R. Armiento,[1] and I. A. Abrikosov[1,3]

[1]*Department of Physics, Chemistry and Biology, Linköping University, SE-581 83 Linköping, Sweden*
[2]*Sandvik Coromant, S-12680 Stockholm, Sweden*
[3]*Materials Modeling and Development Laboratory, National University of Science and Technology 'MISIS', 119049 Moscow, Russia*

(Dated: November 23, 2021)

* henrik.levamaki@liu.se

# I. ELASTIC CONSTANTS

## A. Unrelaxed calculations

Table I: Elastic constants of the unrelaxed B1 calculations before projection to the proper symmetry.

| Alloy | SB | $c_{11}$ | $c_{22}$ | $c_{33}$ | $c_{12}$ | $c_{13}$ | $c_{23}$ | $c_{44}$ | $c_{55}$ | $c_{66}$ | $c_{14}$ | $c_{15}$ | $c_{16}$ | $c_{24}$ | $c_{25}$ | $c_{26}$ | $c_{34}$ | $c_{35}$ | $c_{36}$ | $c_{45}$ | $c_{46}$ | $c_{56}$ |
|---|---|---|---|---|---|---|---|---|---|---|---|---|---|---|---|---|---|---|---|---|---|---|
| AlN | B1 | 440 | 433 | 431 | 173 | 172 | 168 | 308 | 308 | 308 | 0 | 0 | 0 | 0 | 0 | 0 | 0 | 0 | 0 | 0 | 0 | 0 |
| HfN | B1 | 595 | 609 | 595 | 110 | 121 | 110 | 127 | 131 | 127 | −4 | −1 | 3 | 1 | 3 | 1 | 3 | −1 | −4 | −1 | 1 | −1 |
| $Hf_{0.75}Al_{0.25}N$ | B1 | 530 | 524 | 537 | 120 | 111 | 121 | 133 | 136 | 127 | 1 | 4 | 2 | −3 | −1 | 1 | −1 | 3 | 3 | 2 | 3 | −2 |
| $Hf_{0.50}Al_{0.50}N$ | B1 | 478 | 455 | 478 | 128 | 119 | 128 | 141 | 157 | 144 | −2 | 5 | −1 | 5 | 1 | −5 | 3 | 6 | 0 | 0 | 6 | −1 |
| $Hf_{0.25}Al_{0.75}N$ | B1 | 433 | 446 | 441 | 146 | 138 | 141 | 185 | 184 | 182 | 2 | 7 | 4 | −4 | 0 | 3 | −3 | 6 | −3 | −1 | −1 | 1 |
| $Hf_{0.75}Ti_{0.25}N$ | B1 | 589 | 598 | 589 | 106 | 117 | 107 | 137 | 139 | 136 | −2 | 0 | 2 | 0 | 0 | 1 | 0 | 0 | −2 | 0 | −1 | −1 |
| $Hf_{0.50}Ti_{0.50}N$ | B1 | 579 | 594 | 578 | 108 | 118 | 106 | 145 | 149 | 145 | −2 | 1 | 1 | 0 | −1 | 2 | 0 | 1 | −2 | 0 | −1 | 0 |
| $Hf_{0.25}Ti_{0.75}N$ | B1 | 598 | 600 | 597 | 117 | 126 | 118 | 155 | 159 | 155 | 0 | 2 | 1 | 0 | 0 | 1 | 0 | 2 | 0 | 1 | −2 | 1 |
| $Hf_{0.75}Zr_{0.25}N$ | B1 | 579 | 591 | 579 | 105 | 115 | 105 | 127 | 130 | 127 | −3 | 0 | 2 | 0 | 3 | 0 | 2 | 0 | −3 | −1 | 0 | −1 |
| $Hf_{0.50}Zr_{0.50}N$ | B1 | 569 | 578 | 568 | 109 | 119 | 109 | 126 | 129 | 126 | −3 | −1 | 2 | 0 | 1 | 0 | 1 | −1 | −3 | −1 | 0 | −1 |
| $Hf_{0.25}Zr_{0.75}N$ | B1 | 551 | 561 | 551 | 106 | 114 | 106 | 126 | 128 | 126 | −2 | 0 | 1 | 0 | 2 | 0 | 1 | 0 | −2 | −1 | 0 | −1 |
| TiN | B1 | 575 | 583 | 579 | 131 | 138 | 128 | 165 | 165 | 165 | 1 | 3 | −1 | 1 | −7 | 1 | 0 | 3 | 2 | 3 | −3 | 3 |
| $Ti_{0.75}Al_{0.25}N$ | B1 | 534 | 530 | 540 | 138 | 136 | 140 | 177 | 178 | 173 | 0 | 0 | 1 | 0 | 0 | 1 | −1 | 2 | −1 | 1 | 2 | 0 |
| $Ti_{0.50}Al_{0.50}N$ | B1 | 489 | 467 | 494 | 147 | 143 | 151 | 203 | 211 | 201 | −2 | 4 | 0 | 3 | 0 | −3 | 1 | 3 | 4 | 0 | 1 | 0 |
| $Ti_{0.25}Al_{0.75}N$ | B1 | 454 | 457 | 472 | 162 | 160 | 162 | 242 | 240 | 240 | 2 | 4 | 2 | −1 | −2 | 1 | −2 | 5 | −4 | −1 | −2 | 1 |
| ZrN | B1 | 544 | 553 | 544 | 110 | 118 | 110 | 124 | 126 | 124 | −2 | −1 | 1 | 0 | 0 | 0 | 1 | −1 | −2 | −1 | 0 | −1 |
| $Zr_{0.75}Al_{0.25}N$ | B1 | 487 | 484 | 493 | 120 | 112 | 119 | 128 | 131 | 123 | 0 | 0 | 3 | −5 | −4 | 4 | −3 | 1 | 4 | 2 | 2 | −1 |
| $Zr_{0.50}Al_{0.50}N$ | B1 | 444 | 420 | 443 | 128 | 121 | 129 | 138 | 153 | 140 | −2 | 3 | 0 | 4 | 1 | −5 | 3 | 5 | 0 | 0 | 5 | 0 |
| $Zr_{0.25}Al_{0.75}N$ | B1 | 412 | 420 | 421 | 145 | 140 | 138 | 183 | 182 | 181 | 1 | 5 | 5 | −3 | −2 | 3 | −4 | 5 | −3 | −1 | −1 | 0 |
| $Zr_{0.75}Ti_{0.25}N$ | B1 | 539 | 547 | 538 | 105 | 114 | 105 | 131 | 133 | 131 | 0 | 2 | −1 | 2 | 1 | −1 | 2 | 2 | −4 | 0 | −1 | 0 |
| $Zr_{0.50}Ti_{0.50}N$ | B1 | 547 | 556 | 547 | 110 | 121 | 109 | 139 | 142 | 139 | −1 | 0 | 1 | 1 | −2 | 2 | 1 | 0 | −2 | 0 | −2 | 0 |
| $Zr_{0.25}Ti_{0.75}N$ | B1 | 575 | 579 | 574 | 119 | 128 | 120 | 151 | 154 | 151 | −1 | 1 | 1 | 0 | −1 | 1 | 0 | 1 | −1 | 0 | −3 | 0 |

Table II: Elastic constants of the unrelaxed B3 calculations before projection to the proper symmetry.

| Alloy | SB | $c_{11}$ | $c_{22}$ | $c_{33}$ | $c_{12}$ | $c_{13}$ | $c_{23}$ | $c_{44}$ | $c_{55}$ | $c_{66}$ | $c_{14}$ | $c_{15}$ | $c_{16}$ | $c_{24}$ | $c_{25}$ | $c_{26}$ | $c_{34}$ | $c_{35}$ | $c_{36}$ | $c_{45}$ | $c_{46}$ | $c_{56}$ |
|---|---|---|---|---|---|---|---|---|---|---|---|---|---|---|---|---|---|---|---|---|---|---|
| AlN | B3 | 285 | 285 | 285 | 153 | 153 | 153 | 218 | 218 | 218 | 0 | 0 | 0 | 0 | 0 | 0 | 0 | −1 | 0 | 0 | 0 | 0 |
| HfN | B3 | 292 | 290 | 290 | 150 | 153 | 148 | 143 | 143 | 143 | 0 | −1 | 0 | −1 | −1 | −1 | 1 | −1 | 0 | −1 | 1 | −1 |
| $Hf_{0.75}Al_{0.25}N$ | B3 | 269 | 269 | 270 | 141 | 142 | 143 | 132 | 132 | 132 | 1 | 1 | 1 | −1 | −1 | 1 | −1 | 1 | −1 | 1 | 1 | 0 |
| $Hf_{0.50}Al_{0.50}N$ | B3 | 250 | 250 | 251 | 136 | 138 | 136 | 130 | 130 | 131 | 0 | 2 | −1 | 0 | −3 | −1 | 1 | 2 | 0 | 0 | 1 | 1 |
| $Hf_{0.25}Al_{0.75}N$ | B3 | 255 | 256 | 256 | 141 | 143 | 143 | 149 | 149 | 150 | 1 | 2 | 1 | −1 | −2 | 1 | −1 | 1 | −2 | 1 | 1 | −1 |
| $Hf_{0.75}Ti_{0.25}N$ | B3 | 283 | 289 | 283 | 150 | 152 | 150 | 141 | 141 | 141 | 1 | −3 | 0 | 0 | −3 | 0 | 0 | −3 | 0 | −1 | 0 | −1 |
| $Hf_{0.50}Ti_{0.50}N$ | B3 | 286 | 285 | 287 | 151 | 155 | 151 | 138 | 139 | 138 | 0 | 1 | 0 | 0 | 0 | 0 | 0 | 1 | 0 | 0 | 0 | 0 |
| $Hf_{0.25}Ti_{0.75}N$ | B3 | 287 | 287 | 287 | 154 | 154 | 154 | 138 | 138 | 137 | 1 | 0 | −1 | 1 | −1 | −1 | 1 | 0 | −1 | 0 | 0 | 0 |
| $Hf_{0.75}Zr_{0.25}N$ | B3 | 286 | 287 | 287 | 152 | 157 | 153 | 140 | 140 | 140 | 1 | −1 | 1 | −1 | −1 | −1 | 1 | −1 | 1 | −1 | 1 | −1 |
| $Hf_{0.50}Zr_{0.50}N$ | B3 | 270 | 272 | 270 | 145 | 150 | 145 | 134 | 134 | 134 | 1 | 0 | 0 | −1 | 0 | −1 | 0 | 0 | 1 | −1 | 1 | −1 |
| $Hf_{0.25}Zr_{0.75}N$ | B3 | 260 | 263 | 261 | 140 | 146 | 140 | 129 | 129 | 129 | 1 | 2 | 1 | 0 | 2 | 0 | 1 | 2 | 1 | −1 | 1 | −1 |
| TiN | B3 | 290 | 286 | 300 | 151 | 156 | 157 | 138 | 139 | 138 | 0 | 4 | 1 | 1 | 3 | 1 | 1 | 4 | 0 | 1 | 0 | 1 |
| $Ti_{0.75}Al_{0.25}N$ | B3 | 280 | 281 | 280 | 152 | 153 | 153 | 145 | 146 | 144 | 1 | 2 | 1 | −1 | −1 | 1 | −1 | 2 | −1 | 1 | 1 | 0 |
| $Ti_{0.50}Al_{0.50}N$ | B3 | 277 | 276 | 275 | 156 | 158 | 156 | 154 | 156 | 154 | 2 | −1 | 0 | 2 | −6 | −2 | 2 | −1 | −1 | 0 | 1 | 0 |
| $Ti_{0.25}Al_{0.75}N$ | B3 | 270 | 272 | 269 | 151 | 152 | 152 | 174 | 174 | 173 | 0 | 2 | 1 | −1 | −1 | 1 | −1 | 2 | −1 | 1 | 1 | −1 |
| ZrN | B3 | 257 | 259 | 257 | 143 | 149 | 143 | 125 | 125 | 125 | 1 | 0 | 0 | 0 | 0 | 0 | 0 | 0 | 1 | −1 | 1 | −1 |
| $Zr_{0.75}Al_{0.25}N$ | B3 | 245 | 246 | 246 | 140 | 141 | 141 | 118 | 119 | 118 | 1 | 1 | 1 | −1 | −2 | 1 | −1 | 1 | −1 | 1 | 1 | 0 |
| $Zr_{0.50}Al_{0.50}N$ | B3 | 233 | 232 | 234 | 135 | 137 | 135 | 118 | 117 | 118 | 0 | 2 | 0 | 0 | −3 | 0 | 0 | 2 | 0 | 0 | 1 | 0 |
| $Zr_{0.25}Al_{0.75}N$ | B3 | 240 | 241 | 240 | 135 | 137 | 137 | 140 | 140 | 141 | 1 | 1 | 1 | −1 | −2 | 1 | 0 | 1 | −2 | 1 | 1 | −1 |
| $Zr_{0.75}Ti_{0.25}N$ | B3 | 258 | 257 | 259 | 142 | 147 | 141 | 125 | 125 | 125 | 1 | 0 | 0 | 0 | 0 | 0 | 0 | 0 | 1 | −1 | 0 | −1 |
| $Zr_{0.50}Ti_{0.50}N$ | B3 | 265 | 262 | 265 | 145 | 149 | 145 | 126 | 127 | 126 | 0 | −1 | 0 | 0 | −1 | 0 | 0 | −1 | 0 | 0 | 0 | 0 |
| $Zr_{0.25}Ti_{0.75}N$ | B3 | 277 | 275 | 277 | 151 | 152 | 151 | 131 | 132 | 131 | 0 | 0 | 0 | 0 | −1 | 0 | 1 | −1 | 0 | 0 | 0 | 0 |

Table III: Elastic constants of the unrelaxed B4 calculations before projection to the proper symmetry.

| Alloy | SB | $c_{11}$ | $c_{22}$ | $c_{33}$ | $c_{12}$ | $c_{13}$ | $c_{23}$ | $c_{44}$ | $c_{55}$ | $c_{66}$ | $c_{14}$ | $c_{15}$ | $c_{16}$ | $c_{24}$ | $c_{25}$ | $c_{26}$ | $c_{34}$ | $c_{35}$ | $c_{36}$ | $c_{45}$ | $c_{46}$ | $c_{56}$ |
|---|---|---|---|---|---|---|---|---|---|---|---|---|---|---|---|---|---|---|---|---|---|---|
| AlN | B4 | 438 | 440 | 445 | 96 | 61 | 62 | 124 | 124 | 170 | 0 | 0 | −1 | 0 | 0 | −1 | 0 | 0 | −1 | 0 | 0 | 0 |
| HfN | B4 | 305 | 307 | 270 | 129 | 126 | 130 | 55 | 55 | 88 | 0 | 4 | 0 | 0 | 4 | 0 | 0 | 6 | 3 | 0 | 0 | 0 |
| $Hf_{0.75}Al_{0.25}N$ | B4 | 302 | 300 | 275 | 128 | 119 | 121 | 52 | 52 | 86 | 0 | 0 | −1 | 0 | 0 | 0 | 0 | 0 | 0 | 0 | 0 | 0 |
| $Hf_{0.50}Al_{0.50}N$ | B4 | 301 | 299 | 286 | 119 | 105 | 108 | 58 | 55 | 89 | −3 | 0 | −1 | 3 | 1 | 0 | 0 | 0 | 2 | −1 | 0 | −2 |
| $Hf_{0.25}Al_{0.75}N$ | B4 | 332 | 328 | 326 | 108 | 86 | 93 | 75 | 77 | 109 | 0 | −1 | −5 | 0 | −1 | −6 | −1 | 0 | −7 | −1 | 0 | 1 |
| $Hf_{0.75}Ti_{0.25}N$ | B4 | 311 | 309 | 289 | 131 | 133 | 134 | 61 | 62 | 89 | 0 | 1 | −2 | 0 | 1 | −2 | 0 | 1 | 0 | 0 | 0 | 0 |
| $Hf_{0.50}Ti_{0.50}N$ | B4 | 313 | 310 | 298 | 133 | 132 | 132 | 68 | 68 | 90 | −3 | 0 | 0 | 2 | 0 | 0 | 0 | 0 | 1 | 0 | 0 | −2 |
| $Hf_{0.25}Ti_{0.75}N$ | B4 | 308 | 308 | 301 | 130 | 129 | 129 | 73 | 73 | 89 | 0 | 0 | −1 | 0 | 0 | 0 | 0 | 0 | −1 | 0 | 0 | 0 |
| $Hf_{0.75}Zr_{0.25}N$ | B4 | 302 | 305 | 271 | 135 | 130 | 134 | 56 | 55 | 84 | 0 | −1 | 0 | 0 | −1 | 0 | 0 | −1 | 1 | 0 | 0 | 0 |
| $Hf_{0.50}Zr_{0.50}N$ | B4 | 297 | 297 | 271 | 136 | 131 | 133 | 56 | 56 | 80 | 1 | −2 | −2 | 2 | −2 | −1 | 2 | −2 | 0 | 0 | 0 | 0 |
| $Hf_{0.25}Zr_{0.75}N$ | B4 | 284 | 282 | 266 | 129 | 127 | 126 | 56 | 56 | 77 | 0 | 0 | −1 | 0 | 1 | 0 | 0 | 1 | −1 | 0 | 0 | 0 |
| TiN | B4 | 310 | 310 | 303 | 134 | 134 | 133 | 77 | 77 | 89 | 0 | 0 | −1 | 0 | 0 | 1 | 0 | 0 | 0 | −1 | 0 | 0 |
| $Ti_{0.75}Al_{0.25}N$ | B4 | 332 | 328 | 328 | 127 | 121 | 124 | 73 | 73 | 100 | 0 | 0 | −1 | 0 | 0 | 0 | 0 | 0 | 1 | 0 | 0 | 0 |
| $Ti_{0.50}Al_{0.50}N$ | B4 | 343 | 345 | 346 | 118 | 106 | 105 | 79 | 77 | 113 | 0 | −1 | −2 | −1 | 0 | −1 | 0 | 1 | 1 | 0 | 0 | 1 |
| $Ti_{0.25}Al_{0.75}N$ | B4 | 374 | 369 | 377 | 105 | 83 | 85 | 93 | 94 | 132 | 1 | −1 | −2 | 0 | 0 | −1 | 0 | 0 | −1 | 0 | 0 | 0 |
| ZrN | B4 | 278 | 279 | 258 | 130 | 123 | 122 | 58 | 58 | 75 | 0 | 2 | 0 | 0 | 2 | 1 | 0 | 2 | −1 | 0 | 0 | 0 |
| $Zr_{0.75}Al_{0.25}N$ | B4 | 272 | 271 | 262 | 121 | 115 | 117 | 50 | 50 | 75 | 0 | 0 | −1 | −1 | 0 | 1 | −1 | 0 | 0 | −1 | 0 | 0 |
| $Zr_{0.50}Al_{0.50}N$ | B4 | 276 | 274 | 270 | 114 | 102 | 104 | 53 | 50 | 79 | −3 | 0 | −2 | 3 | 1 | 0 | 1 | −1 | 1 | −1 | 0 | −3 |
| $Zr_{0.25}Al_{0.75}N$ | B4 | 314 | 308 | 311 | 105 | 84 | 90 | 70 | 71 | 102 | 0 | −1 | 0 | 0 | 0 | 1 | −2 | 1 | −1 | −1 | 0 | 1 |
| $Zr_{0.75}Ti_{0.25}N$ | B4 | 282 | 284 | 268 | 128 | 122 | 121 | 62 | 62 | 78 | 0 | 0 | −1 | 0 | 0 | 1 | 0 | 0 | −1 | 0 | 0 | 0 |
| $Zr_{0.50}Ti_{0.50}N$ | B4 | 286 | 287 | 274 | 128 | 123 | 122 | 66 | 66 | 79 | −2 | −1 | 0 | 3 | −1 | 1 | 0 | 0 | −1 | 0 | 0 | −2 |
| $Zr_{0.25}Ti_{0.75}N$ | B4 | 291 | 292 | 287 | 127 | 126 | 125 | 71 | 71 | 82 | 0 | −1 | 0 | 0 | −1 | 2 | 1 | 0 | 0 | 0 | 0 | 0 |

## B. Relaxed calculations

Table IV: Elastic constants of the relaxed B1 calculations before projection to the proper symmetry.

| Alloy | SB | $c_{11}$ | $c_{22}$ | $c_{33}$ | $c_{12}$ | $c_{13}$ | $c_{23}$ | $c_{44}$ | $c_{55}$ | $c_{66}$ | $c_{14}$ | $c_{15}$ | $c_{16}$ | $c_{24}$ | $c_{25}$ | $c_{26}$ | $c_{34}$ | $c_{35}$ | $c_{36}$ | $c_{45}$ | $c_{46}$ | $c_{56}$ |
|---|---|---|---|---|---|---|---|---|---|---|---|---|---|---|---|---|---|---|---|---|---|---|
| AlN | B1 | 431 | 429 | 435 | 166 | 169 | 168 | 307 | 307 | 307 | 0 | 0 | 0 | 0 | 0 | 0 | 0 | 0 | 0 | 0 | 0 | 0 |
| HfN | B1 | 594 | 607 | 594 | 108 | 119 | 108 | 127 | 131 | 127 | −4 | −1 | 3 | 1 | 3 | 1 | 3 | −1 | −4 | −1 | 1 | −1 |
| $Hf_{0.75}Al_{0.25}N$ | B1 | 523 | 521 | 529 | 126 | 121 | 126 | 148 | 151 | 142 | 2 | 1 | 0 | −1 | −2 | 0 | 0 | 2 | 0 | 3 | 6 | −3 |
| $Hf_{0.50}Al_{0.50}N$ | B1 | 464 | 445 | 471 | 145 | 138 | 144 | 171 | 182 | 170 | −5 | 0 | 1 | 3 | 2 | −3 | 1 | 1 | 3 | 0 | 11 | 2 |
| $Hf_{0.25}Al_{0.75}N$ | B1 | 424 | 429 | 434 | 158 | 158 | 156 | 220 | 222 | 220 | 0 | 0 | 2 | −2 | 1 | 1 | 0 | 1 | 1 | 4 | 4 | −3 |
| $Hf_{0.75}Ti_{0.25}N$ | B1 | 578 | 584 | 580 | 110 | 118 | 111 | 134 | 136 | 133 | −1 | 1 | 1 | 0 | −1 | 1 | 0 | 0 | −2 | 1 | 0 | −1 |
| $Hf_{0.50}Ti_{0.50}N$ | B1 | 572 | 556 | 575 | 117 | 121 | 118 | 140 | 145 | 140 | −2 | 1 | 2 | 4 | −1 | −3 | −1 | 1 | −1 | 1 | 1 | 0 |
| $Hf_{0.25}Ti_{0.75}N$ | B1 | 577 | 573 | 580 | 118 | 128 | 120 | 153 | 156 | 151 | 0 | 1 | 0 | 1 | −1 | 1 | 1 | 0 | −2 | 1 | −1 | 0 |
| $Hf_{0.75}Zr_{0.25}N$ | B1 | 580 | 591 | 580 | 106 | 116 | 106 | 127 | 131 | 127 | −2 | 0 | 3 | 0 | 1 | 1 | 2 | −1 | −3 | −1 | 0 | −1 |
| $Hf_{0.50}Zr_{0.50}N$ | B1 | 565 | 575 | 566 | 106 | 116 | 104 | 127 | 130 | 127 | −2 | −1 | 2 | 0 | 0 | 1 | 2 | 0 | −2 | −1 | 0 | −1 |
| $Hf_{0.25}Zr_{0.75}N$ | B1 | 551 | 561 | 551 | 103 | 113 | 104 | 126 | 128 | 126 | −2 | 1 | 2 | 0 | 1 | 1 | 1 | 0 | −2 | −1 | 0 | −1 |
| TiN | B1 | 579 | 587 | 585 | 134 | 141 | 132 | 166 | 165 | 166 | 1 | 2 | 0 | 2 | −8 | 2 | 0 | 2 | 2 | 2 | −3 | 2 |
| $Ti_{0.75}Al_{0.25}N$ | B1 | 534 | 529 | 540 | 140 | 136 | 141 | 182 | 183 | 178 | 1 | 0 | 0 | −1 | 0 | −1 | 1 | 0 | 1 | 1 | 1 | 0 |
| $Ti_{0.50}Al_{0.50}N$ | B1 | 502 | 470 | 504 | 158 | 150 | 159 | 212 | 221 | 209 | −2 | 0 | −1 | 2 | 0 | −3 | −1 | −1 | 5 | 0 | 2 | 0 |
| $Ti_{0.25}Al_{0.75}N$ | B1 | 435 | 444 | 450 | 162 | 159 | 162 | 250 | 250 | 248 | 2 | 0 | 0 | 0 | −1 | 1 | 0 | 0 | −2 | 0 | −1 | 0 |
| ZrN | B1 | 541 | 549 | 541 | 108 | 116 | 108 | 125 | 126 | 125 | −1 | −1 | 1 | 1 | 0 | 1 | 1 | −1 | −1 | −1 | 0 | −1 |
| $Zr_{0.75}Al_{0.25}N$ | B1 | 476 | 474 | 482 | 126 | 121 | 125 | 140 | 142 | 134 | 1 | 0 | −1 | 0 | −2 | 0 | 1 | 1 | 0 | 2 | 5 | −1 |
| $Zr_{0.50}Al_{0.50}N$ | B1 | 432 | 411 | 437 | 143 | 137 | 143 | 163 | 174 | 161 | −4 | −1 | 1 | 3 | 2 | −4 | 1 | 0 | 2 | 0 | 10 | 2 |
| $Zr_{0.25}Al_{0.75}N$ | B1 | 408 | 411 | 415 | 158 | 157 | 155 | 214 | 216 | 215 | 0 | −1 | 0 | −1 | 1 | 0 | 1 | 0 | 0 | 3 | 3 | −2 |
| $Zr_{0.75}Ti_{0.25}N$ | B1 | 537 | 541 | 538 | 107 | 117 | 108 | 130 | 131 | 129 | −1 | 0 | 0 | 1 | −1 | 0 | 1 | 0 | −2 | 0 | 0 | −1 |
| $Zr_{0.50}Ti_{0.50}N$ | B1 | 542 | 537 | 542 | 115 | 120 | 113 | 136 | 141 | 137 | −1 | 1 | 3 | 3 | −1 | −2 | −1 | 1 | −1 | 1 | 0 | 0 |
| $Zr_{0.25}Ti_{0.75}N$ | B1 | 568 | 567 | 570 | 119 | 128 | 120 | 150 | 153 | 149 | 0 | 1 | −1 | 0 | −1 | −1 | 1 | 0 | −1 | 1 | −1 | 0 |

Table V: Elastic constants of the relaxed B3 calculations before projection to the proper symmetry.

| Alloy | SB | $c_{11}$ | $c_{22}$ | $c_{33}$ | $c_{12}$ | $c_{13}$ | $c_{23}$ | $c_{44}$ | $c_{55}$ | $c_{66}$ | $c_{14}$ | $c_{15}$ | $c_{16}$ | $c_{24}$ | $c_{25}$ | $c_{26}$ | $c_{34}$ | $c_{35}$ | $c_{36}$ | $c_{45}$ | $c_{46}$ | $c_{56}$ |
|---|---|---|---|---|---|---|---|---|---|---|---|---|---|---|---|---|---|---|---|---|---|---|
| AlN | B3 | 285 | 285 | 285 | 152 | 152 | 152 | 178 | 178 | 178 | 0 | 0 | 0 | 0 | 0 | 0 | 0 | 0 | 0 | 0 | 0 | 0 |
| HfN | B3 | 292 | 293 | 291 | 151 | 154 | 151 | 93 | 94 | 93 | 0 | 0 | 0 | 0 | −1 | 0 | 1 | 0 | 0 | 0 | 0 | 0 |
| $Hf_{0.75}Al_{0.25}N$ | B3 | 274 | 275 | 274 | 144 | 144 | 144 | 100 | 101 | 99 | 2 | 2 | 1 | −1 | −4 | 1 | −1 | 2 | −3 | 2 | 2 | −1 |
| $Hf_{0.50}Al_{0.50}N$ | B3 | 260 | 261 | 263 | 144 | 145 | 143 | 104 | 109 | 104 | −1 | 2 | 0 | −1 | −5 | 0 | −1 | 1 | 1 | −1 | 8 | 1 |
| $Hf_{0.25}Al_{0.75}N$ | B3 | 262 | 262 | 265 | 144 | 143 | 143 | 127 | 127 | 126 | 3 | 0 | 0 | 0 | −2 | 0 | 1 | 0 | −3 | 2 | 7 | −1 |
| $Hf_{0.75}Ti_{0.25}N$ | B3 | 286 | 288 | 287 | 149 | 153 | 148 | 92 | 94 | 92 | 0 | 1 | −1 | 1 | −2 | 0 | 0 | 1 | 0 | 0 | 0 | 0 |
| $Hf_{0.50}Ti_{0.50}N$ | B3 | 286 | 285 | 287 | 149 | 152 | 149 | 92 | 93 | 92 | −1 | 1 | 0 | 0 | −2 | 1 | −1 | 1 | 0 | 0 | 0 | 0 |
| $Hf_{0.25}Ti_{0.75}N$ | B3 | 289 | 288 | 290 | 152 | 153 | 152 | 92 | 92 | 92 | 0 | 0 | −1 | 1 | −2 | 0 | 0 | 0 | −1 | 0 | 0 | 0 |
| $Hf_{0.75}Zr_{0.25}N$ | B3 | 280 | 282 | 280 | 147 | 151 | 147 | 91 | 92 | 91 | 0 | 0 | 0 | 0 | −2 | 0 | 0 | 0 | 0 | 0 | 0 | 0 |
| $Hf_{0.50}Zr_{0.50}N$ | B3 | 272 | 273 | 271 | 145 | 151 | 145 | 89 | 91 | 89 | 0 | 1 | 0 | 0 | −2 | 0 | 0 | 1 | 0 | 0 | 0 | 0 |
| $Hf_{0.25}Zr_{0.75}N$ | B3 | 263 | 265 | 263 | 142 | 148 | 142 | 88 | 89 | 88 | 0 | 0 | 0 | 0 | −1 | 0 | 0 | 0 | 0 | 0 | 0 | 0 |
| TiN | B3 | 293 | 292 | 294 | 156 | 153 | 156 | 90 | 92 | 90 | 0 | 0 | 0 | 0 | −2 | 1 | 0 | 0 | 0 | 0 | 0 | 0 |
| $Ti_{0.75}Al_{0.25}N$ | B3 | 282 | 283 | 282 | 154 | 154 | 154 | 104 | 104 | 102 | 2 | 2 | 1 | −1 | −3 | 1 | −1 | 2 | −3 | 0 | 0 | 0 |
| $Ti_{0.50}Al_{0.50}N$ | B3 | 274 | 275 | 273 | 153 | 155 | 154 | 115 | 118 | 114 | 0 | 2 | 1 | 0 | −4 | 0 | 0 | 2 | 0 | 0 | 2 | 0 |
| $Ti_{0.25}Al_{0.75}N$ | B3 | 272 | 270 | 271 | 151 | 153 | 153 | 139 | 138 | 137 | 2 | 1 | 1 | 0 | −2 | 1 | 0 | 1 | −2 | 1 | 2 | −1 |
| ZrN | B3 | 258 | 259 | 257 | 142 | 149 | 142 | 86 | 87 | 86 | 0 | 0 | −1 | 0 | −1 | 0 | 0 | 0 | 0 | 0 | 0 | 0 |
| $Zr_{0.75}Al_{0.25}N$ | B3 | 247 | 247 | 246 | 141 | 141 | 140 | 92 | 93 | 91 | 3 | 1 | 1 | −1 | −5 | 1 | −1 | 2 | −4 | 1 | 2 | −1 |
| $Zr_{0.50}Al_{0.50}N$ | B3 | 238 | 240 | 242 | 143 | 142 | 142 | 97 | 101 | 96 | −1 | 1 | 0 | 0 | −6 | 0 | 0 | 0 | 1 | −1 | 8 | 0 |
| $Zr_{0.25}Al_{0.75}N$ | B3 | 254 | 250 | 256 | 146 | 145 | 146 | 123 | 122 | 123 | 4 | −1 | −1 | 0 | −4 | −1 | 1 | −1 | −4 | 2 | 6 | −1 |
| $Zr_{0.75}Ti_{0.25}N$ | B3 | 261 | 262 | 262 | 144 | 147 | 143 | 86 | 87 | 86 | 0 | 0 | −1 | 1 | −3 | 0 | 0 | 0 | 0 | 0 | 0 | 0 |
| $Zr_{0.50}Ti_{0.50}N$ | B3 | 270 | 269 | 269 | 147 | 148 | 148 | 88 | 88 | 87 | −1 | 0 | 0 | 1 | −2 | 1 | −1 | 1 | 0 | 0 | 1 | 0 |
| $Zr_{0.25}Ti_{0.75}N$ | B3 | 283 | 281 | 284 | 154 | 154 | 154 | 89 | 89 | 89 | 0 | 0 | −1 | 1 | −2 | 0 | 0 | 0 | −1 | 0 | 1 | 0 |

Table VI: Elastic constants of the relaxed B4 calculations before projection to the proper symmetry.

| Alloy | SB | $c_{11}$ | $c_{22}$ | $c_{33}$ | $c_{12}$ | $c_{13}$ | $c_{23}$ | $c_{44}$ | $c_{55}$ | $c_{66}$ | $c_{14}$ | $c_{15}$ | $c_{16}$ | $c_{24}$ | $c_{25}$ | $c_{26}$ | $c_{34}$ | $c_{35}$ | $c_{36}$ | $c_{45}$ | $c_{46}$ | $c_{56}$ |
|---|---|---|---|---|---|---|---|---|---|---|---|---|---|---|---|---|---|---|---|---|---|---|
| AlN | B4 | 376 | 375 | 352 | 128 | 98 | 98 | 112 | 112 | 123 | 0 | 0 | 0 | 0 | 0 | 0 | 0 | 0 | 0 | 0 | 0 | 0 |
| HfN | B4 | 251 | 252 | 220 | 162 | 162 | 161 | 47 | 47 | 47 | 0 | 0 | 0 | 0 | 0 | 1 | 0 | 0 | 0 | 1 | 0 | 0 |
| $Hf_{0.75}Al_{0.25}N$ | B4 $\rightarrow$ $B_k$ | 295 | 296 | 359 | 205 | 109 | 117 | 104 | 110 | 47 | −1 | 2 | −3 | −1 | −1 | 3 | 0 | 1 | 0 | 0 | −1 | 1 |
| $Hf_{0.50}Al_{0.50}N$ | B4 $\rightarrow$ $B_k$ | 295 | 302 | 110 | 175 | 150 | 141 | 107 | 111 | 60 | 6 | −7 | 6 | −1 | −5 | 4 | −12 | 11 | −1 | −1 | 0 | 3 |
| $Hf_{0.25}Al_{0.75}N$ | B4 | 310 | 295 | 216 | 142 | 125 | 123 | 76 | 97 | 85 | −1 | 0 | 5 | 2 | −1 | −4 | −4 | −5 | 4 | 3 | −5 | 0 |
| $Hf_{0.75}Ti_{0.25}N$ | B4 $\rightarrow$ $B_k$ | 297 | 296 | 493 | 212 | 107 | 104 | 113 | 114 | 45 | 0 | 0 | −1 | 0 | 0 | 5 | 0 | 0 | −3 | 0 | 0 | 0 |
| $Hf_{0.50}Ti_{0.50}N$ | B4 $\rightarrow$ $B_k$ | 301 | 304 | 491 | 211 | 105 | 102 | 120 | 120 | 49 | 0 | 0 | 0 | 0 | 0 | 4 | 0 | −1 | −2 | 0 | 0 | 0 |
| $Hf_{0.25}Ti_{0.75}N$ | B4 $\rightarrow$ $B_k$ | 309 | 311 | 500 | 213 | 107 | 105 | 128 | 129 | 50 | 0 | 0 | 0 | 0 | 0 | 5 | 0 | 0 | −2 | 0 | 0 | 0 |
| $Hf_{0.75}Zr_{0.25}N$ | B4 $\rightarrow$ $B_k$ | 286 | 292 | 495 | 213 | 106 | 103 | 106 | 107 | 43 | 0 | 0 | −1 | 0 | 0 | 7 | 0 | 0 | −3 | −1 | 0 | 0 |
| $Hf_{0.50}Zr_{0.50}N$ | B4 $\rightarrow$ $B_k$ | 283 | 290 | 483 | 207 | 104 | 101 | 107 | 107 | 43 | 0 | 0 | −1 | 0 | 0 | 6 | 0 | 0 | −2 | −1 | 0 | 0 |
| $Hf_{0.25}Zr_{0.75}N$ | B4 $\rightarrow$ $B_k$ | 282 | 289 | 470 | 201 | 103 | 100 | 106 | 107 | 43 | 0 | 0 | 0 | 0 | 0 | 6 | 0 | 0 | −2 | 0 | 0 | 0 |
| TiN | B4 $\rightarrow$ $B_k$ | 316 | 325 | 524 | 220 | 112 | 109 | 139 | 138 | 53 | 0 | 0 | 0 | 0 | 0 | 7 | 0 | 0 | −3 | 0 | 0 | 0 |
| $Ti_{0.75}Al_{0.25}N$ | B4 $\rightarrow$ $B_k$ | 309 | 310 | 438 | 214 | 119 | 120 | 138 | 138 | 51 | 0 | 0 | 1 | 0 | 0 | 1 | 0 | 0 | 1 | −1 | 0 | 0 |
| $Ti_{0.50}Al_{0.50}N$ | B4 $\rightarrow$ $B_k$ | 315 | 313 | 363 | 197 | 127 | 129 | 148 | 147 | 59 | 0 | 0 | 1 | −1 | 0 | 0 | 0 | −1 | 2 | 2 | 0 | 1 |
| $Ti_{0.25}Al_{0.75}N$ | B4 | 319 | 310 | 214 | 136 | 134 | 138 | 87 | 89 | 91 | 6 | 0 | 2 | 0 | −2 | 1 | −10 | 1 | −1 | 0 | −1 | 2 |
| ZrN | B4 $\rightarrow$ $B_k$ | 279 | 290 | 458 | 195 | 103 | 99 | 107 | 106 | 44 | 0 | 0 | 2 | 0 | 0 | 6 | 0 | 0 | −2 | 1 | 0 | 0 |
| $Zr_{0.75}Al_{0.25}N$ | B4 $\rightarrow$ $B_k$ | 276 | 276 | 320 | 196 | 107 | 110 | 99 | 103 | 42 | 0 | 1 | −2 | 0 | −2 | 2 | 0 | 2 | 0 | −2 | −1 | 1 |
| $Zr_{0.50}Al_{0.50}N$ | B4 $\rightarrow$ $B_k$ | 289 | 284 | 202 | 178 | 128 | 123 | 111 | 110 | 55 | −1 | −1 | 4 | −1 | 0 | 2 | −1 | −2 | 1 | 0 | −1 | 1 |
| $Zr_{0.25}Al_{0.75}N$ | B4 | 306 | 298 | 190 | 147 | 116 | 129 | 82 | 95 | 78 | −1 | −2 | 1 | −1 | −4 | −2 | −1 | 3 | 6 | 4 | −2 | 0 |
| $Zr_{0.75}Ti_{0.25}N$ | B4 $\rightarrow$ $B_k$ | 287 | 288 | 453 | 201 | 101 | 100 | 110 | 111 | 44 | 0 | 0 | 0 | 0 | 0 | 4 | 0 | 0 | −2 | 0 | 0 | 0 |
| $Zr_{0.50}Ti_{0.50}N$ | B4 $\rightarrow$ $B_k$ | 295 | 297 | 461 | 205 | 103 | 101 | 116 | 117 | 47 | 0 | 0 | 0 | 0 | 0 | 4 | 0 | −1 | −1 | −1 | 0 | 0 |
| $Zr_{0.25}Ti_{0.75}N$ | B4 $\rightarrow$ $B_k$ | 305 | 308 | 485 | 211 | 106 | 105 | 124 | 126 | 49 | 0 | 0 | 0 | 0 | 0 | 4 | 0 | 0 | −2 | 0 | 0 | 0 |

## II. SQS COORDINATES

B1 $A_{0.25}B_{0.75}N$ POSCAR

```
B36 A12 N48
4.18
2.00000000 2.00000000 0.00000000
0.00000000 2.00000000 2.00000000
1.50000000 0.00000000 1.50000000
A B N
12 36 48
direct
0.75000000 0.00000000 0.66666667 A
0.00000000 0.50000000 0.00000000 A
0.25000000 0.75000000 1.00000000 A
0.50000000 0.25000000 0.00000000 A
0.50000000 0.75000000 1.00000000 A
0.00000000 0.50000000 0.33333333 A
0.25000000 0.75000000 0.33333333 A
0.25000000 0.75000000 0.66666667 A
0.50000000 0.75000000 0.66666667 A
0.75000000 0.50000000 0.33333333 A
0.75000000 0.75000000 0.33333333 A
0.75000000 0.75000000 0.66666667 A
0.00000000 0.00000000 0.00000000 B
0.25000000 0.00000000 0.00000000 B
0.50000000 0.00000000 0.00000000 B
0.75000000 0.00000000 0.00000000 B
0.00000000 0.00000000 0.33333333 B
0.00000000 0.00000000 0.66666667 B
0.25000000 0.00000000 0.33333333 B
0.25000000 0.00000000 0.66666667 B
0.50000000 0.00000000 0.33333333 B
0.50000000 0.00000000 0.66666667 B
0.75000000 0.00000000 0.33333333 B
0.00000000 0.25000000 0.00000000 B
0.00000000 0.75000000 1.00000000 B
0.25000000 0.25000000 0.00000000 B
0.25000000 0.50000000 0.00000000 B
0.50000000 0.50000000 0.00000000 B
0.75000000 0.25000000 0.00000000 B
0.75000000 0.50000000 0.00000000 B
0.75000000 0.75000000 0.00000000 B
0.00000000 0.25000000 0.33333333 B
0.00000000 0.75000000 0.33333333 B
0.00000000 0.25000000 0.66666667 B
0.00000000 0.50000000 0.66666667 B
0.00000000 0.75000000 0.66666667 B
0.25000000 0.25000000 0.33333333 B
0.25000000 0.50000000 0.33333333 B
0.25000000 0.25000000 0.66666667 B
0.25000000 0.50000000 0.66666667 B
0.50000000 0.25000000 0.33333333 B
0.50000000 0.50000000 0.33333333 B
0.50000000 0.75000000 0.33333333 B
0.50000000 0.25000000 0.66666667 B
0.50000000 0.50000000 0.66666667 B
0.75000000 0.25000000 0.33333333 B
```

```
0.75000000 0.25000000 0.66666667 B
0.75000000 0.50000000 0.66666667 B
0.12500000 0.12500000 0.16666667 N
0.37500000 0.12500000 0.16666667 N
0.62500000 0.12500000 0.16666667 N
0.87500000 0.12500000 0.16666667 N
0.12500000 0.12500000 0.50000000 N
0.12500000 0.12500000 0.83333333 N
0.37500000 0.12500000 0.50000000 N
0.37500000 0.12500000 0.83333333 N
0.62500000 0.12500000 0.50000000 N
0.62500000 0.12500000 0.83333333 N
0.87500000 0.12500000 0.50000000 N
0.87500000 0.12500000 0.83333333 N
0.12500000 0.37500000 0.16666667 N
0.12500000 0.62500000 0.16666667 N
0.12500000 0.87500000 0.16666667 N
0.37500000 0.37500000 0.16666667 N
0.37500000 0.62500000 0.16666667 N
0.37500000 0.87500000 0.16666667 N
0.62500000 0.37500000 0.16666667 N
0.62500000 0.62500000 0.16666667 N
0.62500000 0.87500000 0.16666667 N
0.87500000 0.37500000 0.16666667 N
0.87500000 0.62500000 0.16666667 N
0.87500000 0.87500000 0.16666667 N
0.12500000 0.37500000 0.50000000 N
0.12500000 0.62500000 0.50000000 N
0.12500000 0.87500000 0.50000000 N
0.12500000 0.37500000 0.83333333 N
0.12500000 0.62500000 0.83333333 N
0.12500000 0.87500000 0.83333333 N
0.37500000 0.37500000 0.50000000 N
0.37500000 0.62500000 0.50000000 N
0.37500000 0.87500000 0.50000000 N
0.37500000 0.37500000 0.83333333 N
0.37500000 0.62500000 0.83333333 N
0.37500000 0.87500000 0.83333333 N
0.62500000 0.37500000 0.50000000 N
0.62500000 0.62500000 0.50000000 N
0.62500000 0.87500000 0.50000000 N
0.62500000 0.37500000 0.83333333 N
0.62500000 0.62500000 0.83333333 N
0.62500000 0.87500000 0.83333333 N
0.87500000 0.37500000 0.50000000 N
0.87500000 0.62500000 0.50000000 N
0.87500000 0.87500000 0.50000000 N
0.87500000 0.37500000 0.83333333 N
0.87500000 0.62500000 0.83333333 N
0.87500000 0.87500000 0.83333333 N
```

B1 $A_{0.50}B_{0.50}N$ POSCAR

```
A0.5B0.5N
4.18
2.00000000 2.00000000 0.00000000
0.00000000 2.00000000 2.00000000
1.50000000 0.00000000 1.50000000
N B A
48 24 24
D
0.12500000 0.12500000 0.83333333
0.12500000 0.37500000 0.83333333
0.12500000 0.62500000 0.83333333
0.12500000 0.87500000 0.83333333
0.12500000 0.12500000 0.16666667
0.12500000 0.12500000 0.50000000
0.12500000 0.37500000 0.16666667
0.12500000 0.37500000 0.50000000
0.12500000 0.62500000 0.16666667
0.12500000 0.87500000 0.16666667
0.12500000 0.62500000 0.50000000
0.12500000 0.87500000 0.50000000
0.37500000 0.12500000 0.16666667
0.37500000 0.12500000 0.50000000
0.37500000 0.12500000 0.83333333
0.37500000 0.37500000 0.50000000
0.37500000 0.37500000 0.83333333
0.37500000 0.62500000 0.16666667
0.37500000 0.62500000 0.50000000
0.37500000 0.62500000 0.83333333
0.37500000 0.87500000 0.16666667
0.37500000 0.87500000 0.50000000
0.37500000 0.87500000 0.83333333
0.37500000 0.37500000 0.16666667
0.62500000 0.37500000 0.83333333
0.62500000 0.12500000 0.50000000
0.62500000 0.12500000 0.83333333
0.62500000 0.12500000 0.16666667
0.62500000 0.37500000 0.16666667
0.62500000 0.37500000 0.50000000
0.62500000 0.62500000 0.83333333
0.62500000 0.87500000 0.16666667
0.62500000 0.87500000 0.83333333
0.62500000 0.62500000 0.16666667
0.62500000 0.62500000 0.50000000
0.62500000 0.87500000 0.50000000
0.87500000 0.12500000 0.16666667
0.87500000 0.12500000 0.50000000
0.87500000 0.37500000 0.16666667
0.87500000 0.37500000 0.50000000
0.87500000 0.37500000 0.83333333
0.87500000 0.62500000 0.16666667
0.87500000 0.62500000 0.83333333
0.87500000 0.87500000 0.16666667
0.87500000 0.87500000 0.83333333
0.87500000 0.12500000 0.83333333
0.87500000 0.62500000 0.50000000
0.87500000 0.87500000 0.50000000
0.00000000 0.00000000 0.00000000
```

```
0.00000000 0.75000000 0.00000000
0.00000000 0.75000000 0.33333333
0.00000000 1.00000000 0.33333333
0.00000000 0.50000000 0.66666667
0.00000000 0.75000000 0.66666667
0.00000000 1.00000000 0.66666667
0.25000000 0.00000000 0.33333333
0.25000000 0.00000000 0.00000000
0.25000000 0.25000000 0.00000000
0.25000000 0.25000000 0.33333333
0.25000000 0.25000000 0.66666667
0.25000000 0.50000000 0.66666667
0.25000000 1.00000000 0.66666667
0.50000000 0.00000000 0.66666667
0.50000000 0.25000000 0.33333333
0.50000000 0.75000000 0.00000000
0.50000000 0.75000000 0.66666667
0.50000000 1.00000000 0.33333333
0.50000000 0.75000000 0.33333333
0.75000000 0.00000000 0.00000000
0.75000000 0.25000000 0.66666667
0.75000000 0.25000000 0.00000000
0.75000000 0.25000000 0.33333333
0.00000000 0.25000000 0.00000000
0.00000000 0.50000000 0.00000000
0.00000000 0.25000000 0.33333333
0.00000000 0.50000000 0.33333333
0.00000000 0.25000000 0.66666667
0.25000000 0.50000000 0.00000000
0.25000000 0.75000000 0.00000000
0.25000000 0.75000000 0.33333333
0.25000000 0.75000000 0.66666667
0.25000000 0.50000000 0.33333333
0.50000000 0.25000000 0.66666667
0.50000000 0.00000000 0.00000000
0.50000000 0.25000000 0.00000000
0.50000000 0.50000000 0.00000000
0.50000000 0.50000000 0.66666667
0.50000000 0.50000000 0.33333333
0.75000000 0.50000000 0.00000000
0.75000000 0.50000000 0.33333333
0.75000000 0.50000000 0.66666667
0.75000000 0.75000000 0.00000000
0.75000000 0.75000000 0.33333333
0.75000000 0.75000000 0.66666667
0.75000000 1.00000000 0.66666667
0.75000000 1.00000000 0.33333333
```

B1 $A_{0.75}B_{0.25}N$ POSCAR

```
A36 B12 N48
4.18
2.00000000 2.00000000 0.00000000
0.00000000 2.00000000 2.00000000
1.50000000 0.00000000 1.5000000
B A N
12 36 48
direct
0.75000000 0.00000000 0.66666667 B
0.00000000 0.50000000 0.00000000 B
0.25000000 0.75000000 1.00000000 B
0.50000000 0.25000000 0.00000000 B
0.50000000 0.75000000 1.00000000 B
0.00000000 0.50000000 0.33333333 B
0.25000000 0.75000000 0.33333333 B
0.25000000 0.75000000 0.66666667 B
0.50000000 0.75000000 0.66666667 B
0.75000000 0.50000000 0.33333333 B
0.75000000 0.75000000 0.33333333 B
0.75000000 0.75000000 0.66666667 B
0.00000000 0.00000000 0.00000000 A
0.25000000 0.00000000 0.00000000 A
0.50000000 0.00000000 0.00000000 A
0.75000000 0.00000000 0.00000000 A
0.00000000 0.00000000 0.33333333 A
0.00000000 0.00000000 0.66666667 A
0.25000000 0.00000000 0.33333333 A
0.25000000 0.00000000 0.66666667 A
0.50000000 0.00000000 0.33333333 A
0.50000000 0.00000000 0.66666667 A
0.75000000 0.00000000 0.33333333 A
0.00000000 0.25000000 0.00000000 A
0.00000000 0.75000000 1.00000000 A
0.25000000 0.25000000 0.00000000 A
0.25000000 0.50000000 0.00000000 A
0.50000000 0.50000000 0.00000000 A
0.75000000 0.25000000 0.00000000 A
0.75000000 0.50000000 0.00000000 A
0.75000000 0.75000000 0.00000000 A
0.00000000 0.25000000 0.33333333 A
0.00000000 0.75000000 0.33333333 A
0.00000000 0.25000000 0.66666667 A
0.00000000 0.50000000 0.66666667 A
0.00000000 0.75000000 0.66666667 A
0.25000000 0.25000000 0.33333333 A
0.25000000 0.50000000 0.33333333 A
0.25000000 0.25000000 0.66666667 A
0.25000000 0.50000000 0.66666667 A
0.50000000 0.25000000 0.33333333 A
0.50000000 0.50000000 0.33333333 A
0.50000000 0.75000000 0.33333333 A
0.50000000 0.25000000 0.66666667 A
0.50000000 0.50000000 0.66666667 A
0.75000000 0.25000000 0.33333333 A
0.75000000 0.25000000 0.66666667 A
0.75000000 0.50000000 0.66666667 A
0.12500000 0.12500000 0.16666667 N
```

```
0.37500000 0.12500000 0.16666667 N
0.62500000 0.12500000 0.16666667 N
0.87500000 0.12500000 0.16666667 N
0.12500000 0.12500000 0.50000000 N
0.12500000 0.12500000 0.83333333 N
0.37500000 0.12500000 0.50000000 N
0.37500000 0.12500000 0.83333333 N
0.62500000 0.12500000 0.50000000 N
0.62500000 0.12500000 0.83333333 N
0.87500000 0.12500000 0.50000000 N
0.87500000 0.12500000 0.83333333 N
0.12500000 0.37500000 0.16666667 N
0.12500000 0.62500000 0.16666667 N
0.12500000 0.87500000 0.16666667 N
0.37500000 0.37500000 0.16666667 N
0.37500000 0.62500000 0.16666667 N
0.37500000 0.87500000 0.16666667 N
0.62500000 0.37500000 0.16666667 N
0.62500000 0.62500000 0.16666667 N
0.62500000 0.87500000 0.16666667 N
0.87500000 0.37500000 0.16666667 N
0.87500000 0.62500000 0.16666667 N
0.87500000 0.87500000 0.16666667 N
0.12500000 0.37500000 0.50000000 N
0.12500000 0.62500000 0.50000000 N
0.12500000 0.87500000 0.50000000 N
0.12500000 0.37500000 0.83333333 N
0.12500000 0.62500000 0.83333333 N
0.12500000 0.87500000 0.83333333 N
0.37500000 0.37500000 0.50000000 N
0.37500000 0.62500000 0.50000000 N
0.37500000 0.87500000 0.50000000 N
0.37500000 0.37500000 0.83333333 N
0.37500000 0.62500000 0.83333333 N
0.37500000 0.87500000 0.83333333 N
0.62500000 0.37500000 0.50000000 N
0.62500000 0.62500000 0.50000000 N
0.62500000 0.87500000 0.50000000 N
0.62500000 0.37500000 0.83333333 N
0.62500000 0.62500000 0.83333333 N
0.62500000 0.87500000 0.83333333 N
0.87500000 0.37500000 0.50000000 N
0.87500000 0.62500000 0.50000000 N
0.87500000 0.87500000 0.50000000 N
0.87500000 0.37500000 0.83333333 N
0.87500000 0.62500000 0.83333333 N
0.87500000 0.87500000 0.83333333 N
```

B3 $A_{0.25}B_{0.75}N$ POSCAR

```
B36 A12 N48
4.18
2.00000000 2.00000000 0.00000000
0.00000000 2.00000000 2.00000000
1.50000000 0.00000000 1.50000000
A B N
12 36 48
direct
0.75000000 0.00000000 0.66666667 A
0.00000000 0.50000000 0.00000000 A
0.25000000 0.75000000 1.00000000 A
0.50000000 0.25000000 0.00000000 A
0.50000000 0.75000000 1.00000000 A
0.00000000 0.50000000 0.33333333 A
0.25000000 0.75000000 0.33333333 A
0.25000000 0.75000000 0.66666667 A
0.50000000 0.75000000 0.66666667 A
0.75000000 0.50000000 0.33333333 A
0.75000000 0.75000000 0.33333333 A
0.75000000 0.75000000 0.66666667 A
0.00000000 0.00000000 0.00000000 B
0.25000000 0.00000000 0.00000000 B
0.50000000 0.00000000 0.00000000 B
0.75000000 0.00000000 0.00000000 B
0.00000000 0.00000000 0.33333333 B
0.00000000 0.00000000 0.66666667 B
0.25000000 0.00000000 0.33333333 B
0.25000000 0.00000000 0.66666667 B
0.50000000 0.00000000 0.33333333 B
0.50000000 0.00000000 0.66666667 B
0.75000000 0.00000000 0.33333333 B
0.00000000 0.25000000 0.00000000 B
0.00000000 0.75000000 1.00000000 B
0.25000000 0.25000000 0.00000000 B
0.25000000 0.50000000 0.00000000 B
0.50000000 0.50000000 0.00000000 B
0.75000000 0.25000000 0.00000000 B
0.75000000 0.50000000 0.00000000 B
0.75000000 0.75000000 0.00000000 B
0.00000000 0.25000000 0.33333333 B
0.00000000 0.75000000 0.33333333 B
0.00000000 0.25000000 0.66666667 B
0.00000000 0.50000000 0.66666667 B
0.00000000 0.75000000 0.66666667 B
0.25000000 0.25000000 0.33333333 B
0.25000000 0.50000000 0.33333333 B
0.25000000 0.25000000 0.66666667 B
0.25000000 0.50000000 0.66666667 B
0.50000000 0.25000000 0.33333333 B
0.50000000 0.50000000 0.33333333 B
0.50000000 0.75000000 0.33333333 B
0.50000000 0.25000000 0.66666667 B
0.50000000 0.50000000 0.66666667 B
0.75000000 0.25000000 0.33333333 B
0.75000000 0.25000000 0.66666667 B
0.75000000 0.50000000 0.66666667 B
0.06250000 0.06250000 0.08333334 N
```

```
0.31250000 0.06250000 0.08333334 N
0.56250000 0.06250000 0.08333334 N
0.81250000 0.06250000 0.08333334 N
0.06250000 0.06250000 0.41666667 N
0.06250000 0.06250000 0.75000000 N
0.31250000 0.06250000 0.41666667 N
0.31250000 0.06250000 0.75000000 N
0.56250000 0.06250000 0.41666667 N
0.56250000 0.06250000 0.75000000 N
0.81250000 0.06250000 0.41666667 N
0.81250000 0.06250000 0.75000000 N
0.06250000 0.31250000 0.08333334 N
0.06250000 0.56250000 0.08333334 N
0.06250000 0.81250000 0.08333334 N
0.31250000 0.31250000 0.08333334 N
0.31250000 0.56250000 0.08333334 N
0.31250000 0.81250000 0.08333334 N
0.56250000 0.31250000 0.08333334 N
0.56250000 0.56250000 0.08333334 N
0.56250000 0.81250000 0.08333334 N
0.81250000 0.31250000 0.08333334 N
0.81250000 0.56250000 0.08333334 N
0.81250000 0.81250000 0.08333334 N
0.06250000 0.31250000 0.41666667 N
0.06250000 0.56250000 0.41666667 N
0.06250000 0.81250000 0.41666667 N
0.06250000 0.31250000 0.75000000 N
0.06250000 0.56250000 0.75000000 N
0.06250000 0.81250000 0.75000000 N
0.31250000 0.31250000 0.41666667 N
0.31250000 0.56250000 0.41666667 N
0.31250000 0.81250000 0.41666667 N
0.31250000 0.31250000 0.75000000 N
0.31250000 0.56250000 0.75000000 N
0.31250000 0.81250000 0.75000000 N
0.56250000 0.31250000 0.41666667 N
0.56250000 0.56250000 0.41666667 N
0.56250000 0.81250000 0.41666667 N
0.56250000 0.31250000 0.75000000 N
0.56250000 0.56250000 0.75000000 N
0.56250000 0.81250000 0.75000000 N
0.81250000 0.31250000 0.41666667 N
0.81250000 0.56250000 0.41666667 N
0.81250000 0.81250000 0.41666667 N
0.81250000 0.31250000 0.75000000 N
0.81250000 0.56250000 0.75000000 N
0.81250000 0.81250000 0.75000000 N
```

B3 $A_{0.50}B_{0.50}N$ POSCAR

```
A0.5B0.5N
4.18
2.00000000 2.00000000 0.00000000
0.00000000 2.00000000 2.00000000
1.50000000 0.00000000 1.50000000
N B A
48 24 24
D
0.06250000 0.06250000 0.75000000
0.06250000 0.31250000 0.75000000
0.06250000 0.56250000 0.75000000
0.06250000 0.81250000 0.75000000
0.06250000 0.06250000 0.08333334
0.06250000 0.06250000 0.41666667
0.06250000 0.31250000 0.08333334
0.06250000 0.31250000 0.41666667
0.06250000 0.56250000 0.08333334
0.06250000 0.81250000 0.08333334
0.06250000 0.56250000 0.41666667
0.06250000 0.81250000 0.41666667
0.31250000 0.06250000 0.08333334
0.31250000 0.06250000 0.41666667
0.31250000 0.06250000 0.75000000
0.31250000 0.31250000 0.41666667
0.31250000 0.31250000 0.75000000
0.31250000 0.56250000 0.08333334
0.31250000 0.56250000 0.41666667
0.31250000 0.56250000 0.75000000
0.31250000 0.81250000 0.08333334
0.31250000 0.81250000 0.41666667
0.31250000 0.81250000 0.75000000
0.31250000 0.31250000 0.08333334
0.56250000 0.31250000 0.75000000
0.56250000 0.06250000 0.41666667
0.56250000 0.06250000 0.75000000
0.56250000 0.06250000 0.08333334
0.56250000 0.31250000 0.08333334
0.56250000 0.31250000 0.41666667
0.56250000 0.56250000 0.75000000
0.56250000 0.81250000 0.08333334
0.56250000 0.81250000 0.75000000
0.56250000 0.56250000 0.08333334
0.56250000 0.56250000 0.41666667
0.56250000 0.81250000 0.41666667
0.81250000 0.06250000 0.08333334
0.81250000 0.06250000 0.41666667
0.81250000 0.31250000 0.08333334
0.81250000 0.31250000 0.41666667
0.81250000 0.31250000 0.75000000
0.81250000 0.56250000 0.08333334
0.81250000 0.56250000 0.75000000
0.81250000 0.81250000 0.08333334
0.81250000 0.81250000 0.75000000
0.81250000 0.06250000 0.75000000
0.81250000 0.56250000 0.41666667
0.81250000 0.81250000 0.41666667
0.00000000 0.00000000 0.00000000
```

```
0.00000000 0.75000000 0.00000000
0.00000000 0.75000000 0.33333333
0.00000000 1.00000000 0.33333333
0.00000000 0.50000000 0.66666667
0.00000000 0.75000000 0.66666667
0.00000000 1.00000000 0.66666667
0.25000000 0.00000000 0.33333333
0.25000000 0.00000000 0.00000000
0.25000000 0.25000000 0.00000000
0.25000000 0.25000000 0.33333333
0.25000000 0.25000000 0.66666667
0.25000000 0.50000000 0.66666667
0.25000000 1.00000000 0.66666667
0.50000000 0.00000000 0.66666667
0.50000000 0.25000000 0.33333333
0.50000000 0.75000000 0.00000000
0.50000000 0.75000000 0.66666667
0.50000000 1.00000000 0.33333333
0.50000000 0.75000000 0.33333333
0.75000000 0.00000000 0.00000000
0.75000000 0.25000000 0.66666667
0.75000000 0.25000000 0.00000000
0.75000000 0.25000000 0.33333333
0.00000000 0.25000000 0.00000000
0.00000000 0.50000000 0.00000000
0.00000000 0.25000000 0.33333333
0.00000000 0.50000000 0.33333333
0.00000000 0.25000000 0.66666667
0.25000000 0.50000000 0.00000000
0.25000000 0.75000000 0.00000000
0.25000000 0.75000000 0.33333333
0.25000000 0.75000000 0.66666667
0.25000000 0.50000000 0.33333333
0.50000000 0.25000000 0.66666667
0.50000000 0.00000000 0.00000000
0.50000000 0.25000000 0.00000000
0.50000000 0.50000000 0.00000000
0.50000000 0.50000000 0.66666667
0.50000000 0.50000000 0.33333333
0.75000000 0.50000000 0.00000000
0.75000000 0.50000000 0.33333333
0.75000000 0.50000000 0.66666667
0.75000000 0.75000000 0.00000000
0.75000000 0.75000000 0.33333333
0.75000000 0.75000000 0.66666667
0.75000000 1.00000000 0.66666667
0.75000000 1.00000000 0.33333333
```

B3 $A_{0.75}B_{0.25}N$ POSCAR

```
A36 B12 N48
4.18
2.00000000 2.00000000 0.00000000
0.00000000 2.00000000 2.00000000
1.50000000 0.00000000 1.5000000
B A N
12 36 48
direct
0.75000000 0.00000000 0.66666667 B
0.00000000 0.50000000 0.00000000 B
0.25000000 0.75000000 1.00000000 B
0.50000000 0.25000000 0.00000000 B
0.50000000 0.75000000 1.00000000 B
0.00000000 0.50000000 0.33333333 B
0.25000000 0.75000000 0.33333333 B
0.25000000 0.75000000 0.66666667 B
0.50000000 0.75000000 0.66666667 B
0.75000000 0.50000000 0.33333333 B
0.75000000 0.75000000 0.33333333 B
0.75000000 0.75000000 0.66666667 B
0.00000000 0.00000000 0.00000000 A
0.25000000 0.00000000 0.00000000 A
0.50000000 0.00000000 0.00000000 A
0.75000000 0.00000000 0.00000000 A
0.00000000 0.00000000 0.33333333 A
0.00000000 0.00000000 0.66666667 A
0.25000000 0.00000000 0.33333333 A
0.25000000 0.00000000 0.66666667 A
0.50000000 0.00000000 0.33333333 A
0.50000000 0.00000000 0.66666667 A
0.75000000 0.00000000 0.33333333 A
0.00000000 0.25000000 0.00000000 A
0.00000000 0.75000000 1.00000000 A
0.25000000 0.25000000 0.00000000 A
0.25000000 0.50000000 0.00000000 A
0.50000000 0.50000000 0.00000000 A
0.75000000 0.25000000 0.00000000 A
0.75000000 0.50000000 0.00000000 A
0.75000000 0.75000000 0.00000000 A
0.00000000 0.25000000 0.33333333 A
0.00000000 0.75000000 0.33333333 A
0.00000000 0.25000000 0.66666667 A
0.00000000 0.50000000 0.66666667 A
0.00000000 0.75000000 0.66666667 A
0.25000000 0.25000000 0.33333333 A
0.25000000 0.50000000 0.33333333 A
0.25000000 0.25000000 0.66666667 A
0.25000000 0.50000000 0.66666667 A
0.50000000 0.25000000 0.33333333 A
0.50000000 0.50000000 0.33333333 A
0.50000000 0.75000000 0.33333333 A
0.50000000 0.25000000 0.66666667 A
0.50000000 0.50000000 0.66666667 A
0.75000000 0.25000000 0.33333333 A
0.75000000 0.25000000 0.66666667 A
0.75000000 0.50000000 0.66666667 A
0.06250000 0.06250000 0.08333334 N
```

```
0.31250000 0.06250000 0.08333334 N
0.56250000 0.06250000 0.08333334 N
0.81250000 0.06250000 0.08333334 N
0.06250000 0.06250000 0.41666667 N
0.06250000 0.06250000 0.75000000 N
0.31250000 0.06250000 0.41666667 N
0.31250000 0.06250000 0.75000000 N
0.56250000 0.06250000 0.41666667 N
0.56250000 0.06250000 0.75000000 N
0.81250000 0.06250000 0.41666667 N
0.81250000 0.06250000 0.75000000 N
0.06250000 0.31250000 0.08333334 N
0.06250000 0.56250000 0.08333334 N
0.06250000 0.81250000 0.08333334 N
0.31250000 0.31250000 0.08333334 N
0.31250000 0.56250000 0.08333334 N
0.31250000 0.81250000 0.08333334 N
0.56250000 0.31250000 0.08333334 N
0.56250000 0.56250000 0.08333334 N
0.56250000 0.81250000 0.08333334 N
0.81250000 0.31250000 0.08333334 N
0.81250000 0.56250000 0.08333334 N
0.81250000 0.81250000 0.08333334 N
0.06250000 0.31250000 0.41666667 N
0.06250000 0.56250000 0.41666667 N
0.06250000 0.81250000 0.41666667 N
0.06250000 0.31250000 0.75000000 N
0.06250000 0.56250000 0.75000000 N
0.06250000 0.81250000 0.75000000 N
0.31250000 0.31250000 0.41666667 N
0.31250000 0.56250000 0.41666667 N
0.31250000 0.81250000 0.41666667 N
0.31250000 0.31250000 0.75000000 N
0.31250000 0.56250000 0.75000000 N
0.31250000 0.81250000 0.75000000 N
0.56250000 0.31250000 0.41666667 N
0.56250000 0.56250000 0.41666667 N
0.56250000 0.81250000 0.41666667 N
0.56250000 0.31250000 0.75000000 N
0.56250000 0.56250000 0.75000000 N
0.56250000 0.81250000 0.75000000 N
0.81250000 0.31250000 0.41666667 N
0.81250000 0.56250000 0.41666667 N
0.81250000 0.81250000 0.41666667 N
0.81250000 0.31250000 0.75000000 N
0.81250000 0.56250000 0.75000000 N
0.81250000 0.81250000 0.75000000 N
```

B4 $A_{0.25}B_{0.75}N$ POSCAR

```
A12 B36 N48
4.0
-3.50000000 0.86602500 0.00000000
2.50000000 -2.59807500 0.00000000
0.00000000 0.00000000 4.89897900
A B N
12 36 48
direct
0.16666675 0.83333325 1.00000000 A
0.79166675 0.70833325 1.00000000 A
0.66666675 0.33333325 0.33333333 A
0.29166675 0.20833325 0.33333333 A
0.16666675 0.83333325 0.66666667 A
0.79166675 0.70833325 0.66666667 A
0.58333325 0.41666675 0.50000000 A
0.20833325 0.29166675 0.50000000 A
0.83333325 0.16666675 0.50000000 A
0.08333325 0.91666675 0.50000000 A
0.95833325 0.54166675 0.83333333 A
0.83333325 0.16666675 0.83333333 A
0.41666675 0.58333325 1.00000000 B
0.04166675 0.45833325 1.00000000 B
0.66666675 0.33333325 1.00000000 B
0.29166675 0.20833325 1.00000000 B
0.91666675 0.08333325 1.00000000 B
0.54166675 0.95833325 1.00000000 B
0.41666675 0.58333325 0.33333333 B
0.04166675 0.45833325 0.33333333 B
0.91666675 0.08333325 0.33333333 B
0.54166675 0.95833325 0.33333333 B
0.16666675 0.83333325 0.33333333 B
0.79166675 0.70833325 0.33333333 B
0.41666675 0.58333325 0.66666667 B
0.04166675 0.45833325 0.66666667 B
0.66666675 0.33333325 0.66666667 B
0.29166675 0.20833325 0.66666667 B
0.91666675 0.08333325 0.66666667 B
0.54166675 0.95833325 0.66666667 B
0.33333325 0.66666675 0.16666667 B
0.95833325 0.54166675 0.16666667 B
0.58333325 0.41666675 0.16666667 B
0.20833325 0.29166675 0.16666667 B
0.83333325 0.16666675 0.16666667 B
0.45833325 0.04166675 0.16666667 B
0.08333325 0.91666675 0.16666667 B
0.70833325 0.79166675 0.16666667 B
0.33333325 0.66666675 0.50000000 B
0.95833325 0.54166675 0.50000000 B
0.45833325 0.04166675 0.50000000 B
0.70833325 0.79166675 0.50000000 B
0.33333325 0.66666675 0.83333333 B
0.58333325 0.41666675 0.83333333 B
0.20833325 0.29166675 0.83333333 B
0.45833325 0.04166675 0.83333333 B
0.08333325 0.91666675 0.83333333 B
0.70833325 0.79166675 0.83333333 B
0.41666675 0.58333325 0.12666667 N
```

```
0.04166675 0.45833325 0.12666667 N
0.66666675 0.33333325 0.12666667 N
0.29166675 0.20833325 0.12666667 N
0.91666675 0.08333325 0.12666667 N
0.54166675 0.95833325 0.12666667 N
0.16666675 0.83333325 0.12666667 N
0.79166675 0.70833325 0.12666667 N
0.41666675 0.58333325 0.46000000 N
0.04166675 0.45833325 0.46000000 N
0.66666675 0.33333325 0.46000000 N
0.29166675 0.20833325 0.46000000 N
0.91666675 0.08333325 0.46000000 N
0.54166675 0.95833325 0.46000000 N
0.16666675 0.83333325 0.46000000 N
0.79166675 0.70833325 0.46000000 N
0.41666675 0.58333325 0.79333333 N
0.04166675 0.45833325 0.79333333 N
0.66666675 0.33333325 0.79333333 N
0.29166675 0.20833325 0.79333333 N
0.91666675 0.08333325 0.79333333 N
0.54166675 0.95833325 0.79333333 N
0.16666675 0.83333325 0.79333333 N
0.79166675 0.70833325 0.79333333 N
0.33333325 0.66666675 0.29333333 N
0.95833325 0.54166675 0.29333333 N
0.58333325 0.41666675 0.29333333 N
0.20833325 0.29166675 0.29333333 N
0.83333325 0.16666675 0.29333333 N
0.45833325 0.04166675 0.29333333 N
0.08333325 0.91666675 0.29333333 N
0.70833325 0.79166675 0.29333333 N
0.33333325 0.66666675 0.62666667 N
0.95833325 0.54166675 0.62666667 N
0.58333325 0.41666675 0.62666667 N
0.20833325 0.29166675 0.62666667 N
0.83333325 0.16666675 0.62666667 N
0.45833325 0.04166675 0.62666667 N
0.08333325 0.91666675 0.62666667 N
0.70833325 0.79166675 0.62666667 N
0.33333325 0.66666675 0.96000000 N
0.95833325 0.54166675 0.96000000 N
0.58333325 0.41666675 0.96000000 N
0.20833325 0.29166675 0.96000000 N
0.83333325 0.16666675 0.96000000 N
0.45833325 0.04166675 0.96000000 N
0.08333325 0.91666675 0.96000000 N
0.70833325 0.79166675 0.96000000 N
```

B4 $A_{0.50}B_{0.50}N$ POSCAR

```
A24 B24 N48
4.0
-3.50000000 0.86602500 0.00000000
2.50000000 -2.59807500 0.00000000
0.00000000 0.00000000 4.89897900
A B N
24 24 48
direct
0.66666675 0.33333325 1.00000000 A
0.29166675 0.20833325 1.00000000 A
0.91666675 0.08333325 1.00000000 A
0.79166675 0.70833325 1.00000000 A
0.41666675 0.58333325 0.33333333 A
0.04166675 0.45833325 0.33333333 A
0.91666675 0.08333325 0.33333333 A
0.54166675 0.95833325 0.33333333 A
0.16666675 0.83333325 0.33333333 A
0.79166675 0.70833325 0.33333333 A
0.04166675 0.45833325 0.66666667 A
0.29166675 0.20833325 0.66666667 A
0.91666675 0.08333325 0.66666667 A
0.16666675 0.83333325 0.66666667 A
0.33333325 0.66666675 0.16666667 A
0.58333325 0.41666675 0.16666667 A
0.70833325 0.79166675 0.16666667 A
0.33333325 0.66666675 0.50000000 A
0.58333325 0.41666675 0.50000000 A
0.20833325 0.29166675 0.50000000 A
0.08333325 0.91666675 0.50000000 A
0.70833325 0.79166675 0.50000000 A
0.83333325 0.16666675 0.83333333 A
0.70833325 0.79166675 0.83333333 A
0.41666675 0.58333325 1.00000000 B
0.04166675 0.45833325 1.00000000 B
0.54166675 0.95833325 1.00000000 B
0.16666675 0.83333325 1.00000000 B
0.66666675 0.33333325 0.33333333 B
0.29166675 0.20833325 0.33333333 B
0.41666675 0.58333325 0.66666667 B
0.66666675 0.33333325 0.66666667 B
0.54166675 0.95833325 0.66666667 B
0.79166675 0.70833325 0.66666667 B
0.95833325 0.54166675 0.16666667 B
0.20833325 0.29166675 0.16666667 B
0.83333325 0.16666675 0.16666667 B
0.45833325 0.04166675 0.16666667 B
0.08333325 0.91666675 0.16666667 B
0.95833325 0.54166675 0.50000000 B
0.83333325 0.16666675 0.50000000 B
0.45833325 0.04166675 0.50000000 B
0.33333325 0.66666675 0.83333333 B
0.95833325 0.54166675 0.83333333 B
0.58333325 0.41666675 0.83333333 B
0.20833325 0.29166675 0.83333333 B
0.45833325 0.04166675 0.83333333 B
0.08333325 0.91666675 0.83333333 B
0.41666675 0.58333325 0.12666667 N
```

```
0.04166675 0.45833325 0.12666667 N
0.66666675 0.33333325 0.12666667 N
0.29166675 0.20833325 0.12666667 N
0.91666675 0.08333325 0.12666667 N
0.54166675 0.95833325 0.12666667 N
0.16666675 0.83333325 0.12666667 N
0.79166675 0.70833325 0.12666667 N
0.41666675 0.58333325 0.46000000 N
0.04166675 0.45833325 0.46000000 N
0.66666675 0.33333325 0.46000000 N
0.29166675 0.20833325 0.46000000 N
0.91666675 0.08333325 0.46000000 N
0.54166675 0.95833325 0.46000000 N
0.16666675 0.83333325 0.46000000 N
0.79166675 0.70833325 0.46000000 N
0.41666675 0.58333325 0.79333333 N
0.04166675 0.45833325 0.79333333 N
0.66666675 0.33333325 0.79333333 N
0.29166675 0.20833325 0.79333333 N
0.91666675 0.08333325 0.79333333 N
0.54166675 0.95833325 0.79333333 N
0.16666675 0.83333325 0.79333333 N
0.79166675 0.70833325 0.79333333 N
0.33333325 0.66666675 0.29333333 N
0.95833325 0.54166675 0.29333333 N
0.58333325 0.41666675 0.29333333 N
0.20833325 0.29166675 0.29333333 N
0.83333325 0.16666675 0.29333333 N
0.45833325 0.04166675 0.29333333 N
0.08333325 0.91666675 0.29333333 N
0.70833325 0.79166675 0.29333333 N
0.33333325 0.66666675 0.62666667 N
0.95833325 0.54166675 0.62666667 N
0.58333325 0.41666675 0.62666667 N
0.20833325 0.29166675 0.62666667 N
0.83333325 0.16666675 0.62666667 N
0.45833325 0.04166675 0.62666667 N
0.08333325 0.91666675 0.62666667 N
0.70833325 0.79166675 0.62666667 N
0.33333325 0.66666675 0.96000000 N
0.95833325 0.54166675 0.96000000 N
0.58333325 0.41666675 0.96000000 N
0.20833325 0.29166675 0.96000000 N
0.83333325 0.16666675 0.96000000 N
0.45833325 0.04166675 0.96000000 N
0.08333325 0.91666675 0.96000000 N
0.70833325 0.79166675 0.96000000 N
```

B4 $A_{0.75}B_{0.25}N$ POSCAR

```
B12 A36 N48
4.0
-3.50000000 0.86602500 0.00000000
2.50000000 -2.59807500 0.00000000
0.00000000 0.00000000 4.89897900
B A N
12 36 48
direct
0.16666675 0.83333325 1.00000000 B
0.79166675 0.70833325 1.00000000 B
0.66666675 0.33333325 0.33333333 B
0.29166675 0.20833325 0.33333333 B
0.16666675 0.83333325 0.66666667 B
0.79166675 0.70833325 0.66666667 B
0.58333325 0.41666675 0.50000000 B
0.20833325 0.29166675 0.50000000 B
0.83333325 0.16666675 0.50000000 B
0.08333325 0.91666675 0.50000000 B
0.95833325 0.54166675 0.83333333 B
0.83333325 0.16666675 0.83333333 B
0.41666675 0.58333325 1.00000000 A
0.04166675 0.45833325 1.00000000 A
0.66666675 0.33333325 1.00000000 A
0.29166675 0.20833325 1.00000000 A
0.91666675 0.08333325 1.00000000 A
0.54166675 0.95833325 1.00000000 A
0.41666675 0.58333325 0.33333333 A
0.04166675 0.45833325 0.33333333 A
0.91666675 0.08333325 0.33333333 A
0.54166675 0.95833325 0.33333333 A
0.16666675 0.83333325 0.33333333 A
0.79166675 0.70833325 0.33333333 A
0.41666675 0.58333325 0.66666667 A
0.04166675 0.45833325 0.66666667 A
0.66666675 0.33333325 0.66666667 A
0.29166675 0.20833325 0.66666667 A
0.91666675 0.08333325 0.66666667 A
0.54166675 0.95833325 0.66666667 A
0.33333325 0.66666675 0.16666667 A
0.95833325 0.54166675 0.16666667 A
0.58333325 0.41666675 0.16666667 A
0.20833325 0.29166675 0.16666667 A
0.83333325 0.16666675 0.16666667 A
0.45833325 0.04166675 0.16666667 A
0.08333325 0.91666675 0.16666667 A
0.70833325 0.79166675 0.16666667 A
0.33333325 0.66666675 0.50000000 A
0.95833325 0.54166675 0.50000000 A
0.45833325 0.04166675 0.50000000 A
0.70833325 0.79166675 0.50000000 A
0.33333325 0.66666675 0.83333333 A
0.58333325 0.41666675 0.83333333 A
0.20833325 0.29166675 0.83333333 A
0.45833325 0.04166675 0.83333333 A
0.08333325 0.91666675 0.83333333 A
0.70833325 0.79166675 0.83333333 A
0.41666675 0.58333325 0.12666667 N
```

```
0.04166675 0.45833325 0.12666667 N
0.66666675 0.33333325 0.12666667 N
0.29166675 0.20833325 0.12666667 N
0.91666675 0.08333325 0.12666667 N
0.54166675 0.95833325 0.12666667 N
0.16666675 0.83333325 0.12666667 N
0.79166675 0.70833325 0.12666667 N
0.41666675 0.58333325 0.46000000 N
0.04166675 0.45833325 0.46000000 N
0.66666675 0.33333325 0.46000000 N
0.29166675 0.20833325 0.46000000 N
0.91666675 0.08333325 0.46000000 N
0.54166675 0.95833325 0.46000000 N
0.16666675 0.83333325 0.46000000 N
0.79166675 0.70833325 0.46000000 N
0.41666675 0.58333325 0.79333333 N
0.04166675 0.45833325 0.79333333 N
0.66666675 0.33333325 0.79333333 N
0.29166675 0.20833325 0.79333333 N
0.91666675 0.08333325 0.79333333 N
0.54166675 0.95833325 0.79333333 N
0.16666675 0.83333325 0.79333333 N
0.79166675 0.70833325 0.79333333 N
0.33333325 0.66666675 0.29333333 N
0.95833325 0.54166675 0.29333333 N
0.58333325 0.41666675 0.29333333 N
0.20833325 0.29166675 0.29333333 N
0.83333325 0.16666675 0.29333333 N
0.45833325 0.04166675 0.29333333 N
0.08333325 0.91666675 0.29333333 N
0.70833325 0.79166675 0.29333333 N
0.33333325 0.66666675 0.62666667 N
0.95833325 0.54166675 0.62666667 N
0.58333325 0.41666675 0.62666667 N
0.20833325 0.29166675 0.62666667 N
0.83333325 0.16666675 0.62666667 N
0.45833325 0.04166675 0.62666667 N
0.08333325 0.91666675 0.62666667 N
0.70833325 0.79166675 0.62666667 N
0.33333325 0.66666675 0.96000000 N
0.95833325 0.54166675 0.96000000 N
0.58333325 0.41666675 0.96000000 N
0.20833325 0.29166675 0.96000000 N
0.83333325 0.16666675 0.96000000 N
0.45833325 0.04166675 0.96000000 N
0.08333325 0.91666675 0.96000000 N
0.70833325 0.79166675 0.96000000 N
```
